# Supplementary material for: Revisiting the Impact of Dependency Network Metrics on Software Defect Prediction
Source: arXiv:2202.06145 source file (2022-02-12)
Supplement: Supplementary file 1 [file appendix.tex]

%\section{Overview of the Double SK-ESD test}~\label{sec:app1}

 % \begin{figure*}[!htbp]
 % \noindent\begin{minipage}{\textwidth}
%\centering

%\includegraphics[angle=90,width=6in]{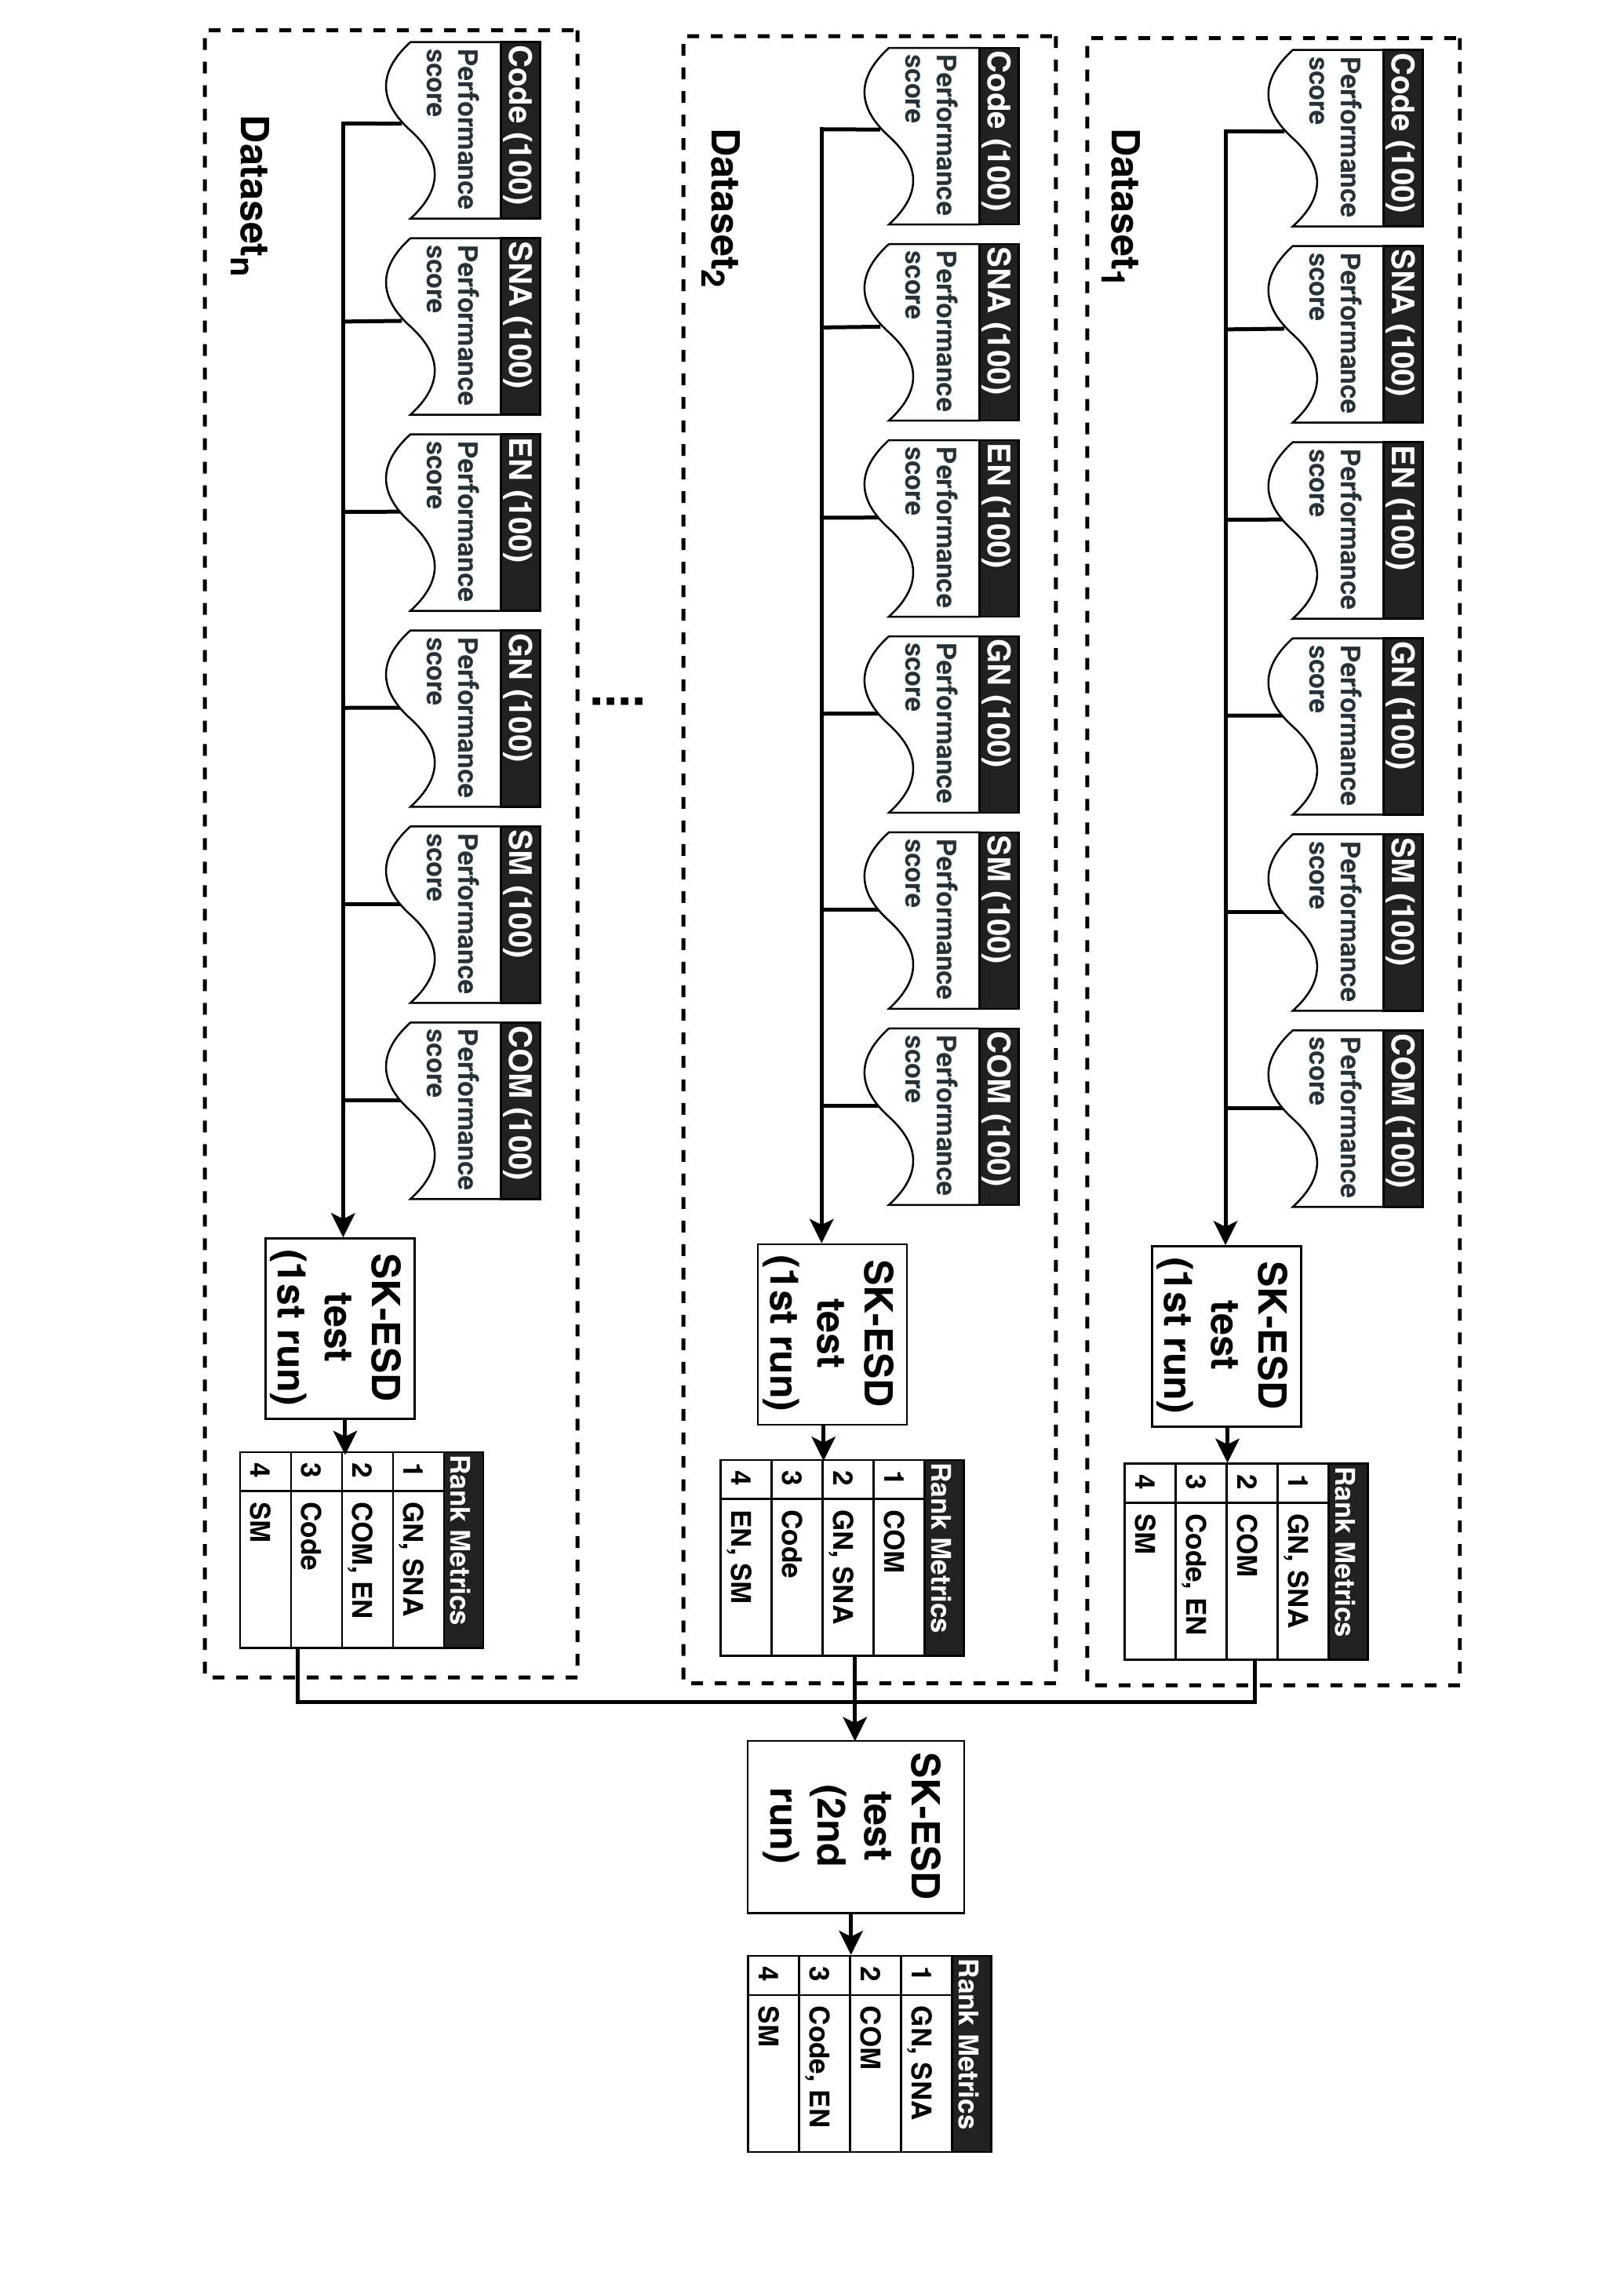}
%\caption{Overview of our Double Sk-ESD test}\label{fig:ESD}
%\captionof{figure}{Overview of our Double Sk-ESD test}\label{fig:ESD}
%\end{minipage}
%\end{figure*}

\section{Details about each of the studied SNA metrics}~\label{sec:app1}
Table~\ref{table:SNAmetric} gives a more details about each of the studied SNA metrics used in Section 3.1.2.

\begin{table*}[!htb]
\centering
\caption{Description about each of the studied SNA metrics}\label{table:SNAmetric}
\hspace{0.5cm}
\centering
 \begin{tabular} {l|p{50pt}|p{300pt}} 
\hline
\textbf{Metric family}&\textbf{Measure}&\textbf{Description}\\
\hline
\multirow{12}{*}{\textbf{EN metrics}}&\textbf{Size} & The number of nodes in the ego network of the given module\\
\cline{2-3}
&\textbf{Ties} & The number of edges in the ego network of the given module\\
\cline{2-3}
&\textbf{Pairs} & The number of unique pairs of nodes in ego network of the given module, i.e., $Size \times (Size-1)$\\
\cline{2-3}
&\textbf{Density} & The percentage of possible ties that are actually present, i.e., $Ties/Pairs$\\
\cline{2-3}
&\textbf{WeakComp} & The number of weak components in neighborhood of the given module\\
\cline{2-3}
&\textbf{nWeakComp} & The number of weak components normalized by size of the module, i.e., $WeakComp/Size$\\
\cline{2-3}
&\textbf{2StepReach} & The percentage of nodes that are reachable within two steps from the given node in a ego network\\
\cline{2-3}
&\textbf{ReachEfficency} & Normalize 2StepReach by Size, i.e., $2StepReach/Size$ \\
\cline{2-3}
&\textbf{Brokerage} & The number of pairs that are not directly connected to the given module.\\
\cline{2-3}
&\textbf{nBrokerage} & Normalize Brokerage by the number of pairs, i.e.,$Brokerage/Pairs$\\
\cline{2-3}
&\textbf{EgoBetween} & The percentage of shortest paths between any two nodes in the ego network \\
\cline{2-3}
&\textbf{nEgoBetween} & Normalize Betweenness  by the size of the ego network of the given node.\\
\hline
\multirow{11}{*}{\textbf{GN metrics}}&\textbf{Degree} & The number of nodes that are directly connected to a given node.\\
\cline{2-3}
&\textbf{Eigenvector} & Assign relative scores to all nodes in the dependency graphs similar to Google's PageRank. The node that is connected to many highly connected neighbours would have higher value and vice versa.\\
\cline{2-3}
&\textbf{power} & A modification of the degree of centrality measure, which measures the connections of the nodes in its neighborhood.\\
\cline{2-3}
&\textbf{Closeness} & Sum of the lengths of the shortest paths from a node to all other nodes in the Global network. \\
\cline{2-3}
&\textbf{Betweenness} & Measures how often a node occurs in shortest paths between any two nodes in the Global network.\\
\cline{2-3}
&\textbf{Information} & The harmonic mean of the length of all paths leading to the node.\\
\cline{2-3}
&\textbf{dwReach} & The number of nodes that can be reached from a node. \\
\cline{2-3}
&\textbf{EffSize} & The number of nodes that are connected to a node minus the average number of ties between these nodes.\\
\cline{2-3}
&\textbf{Efficiency} & Normalize EffSize to the total size of the global network.\\
\cline{2-3}
&\textbf{Constraint} & Measures the extent to which the node is limited in options to reach other nodes.\\
\cline{2-3}
&\textbf{Hierarchy} & Measures the concentration of constraint in the global network.\\
\hline
\end{tabular}
\end{table*}

\section{Performance measures used in the Defect-classification scenario}~\label{sec:app2}
Table~\ref{table:measures} presents a detailed description about each of the studied performance measure used in Section 3.3.2.

\begin{table*}[!htb]
\centering
\caption{Performance measures used in our study on the Defect-classification scenario}\label{table:measures}
\hspace{0.5cm}
\centering
 \begin{tabular} {l|p{180pt}|p{200pt}} 
\hline
\textbf{Measure}&\textbf{Definition}&\textbf{Description}\\
\hline
AUC&The  area  under  the  receiver  operator  characteristic  Curve.& The  receiver  operator  characteristic  Curve plots the true positive rate against the false positive rate across all the thresholds\\
Recall&$Recall=\frac{TP}{TP+FN}$& The percentage of defective modules that are correctly classified as defective.\\
Precision&$Precision=\frac{TP}{TP+FP}$&The percentage of predicted defective modules that are actually defective.\\
MCC&$MCC=\frac{TP\times TN-FP\times FN}{(TP+FP)(TP+FN)(TN+FP)(TN+FN)}$& A more balanced indicator which considers TP, TN, FP and FN.\\
Brier score&$Brier=\frac{1}{N}\sum_{i=1}^{N}(p_{i}-y_{i})^{2}$&A measure of the  mean  squared  difference  between  the  predicted  probability assigned  to a module and the actual probability.\\
\hline
\end{tabular}
\end{table*}

\section{Performance of the models trained on the studied metrics in the Within-project context}~\label{sec:app3}
Figure~\ref{fig:withip} gives a detailed overview of the performance of models trained on different metric families across the studied datasets for all the SDP scenarios in the Within-project context.

\begin{figure*}[!htbp]
\centering
\includegraphics[width=7in]{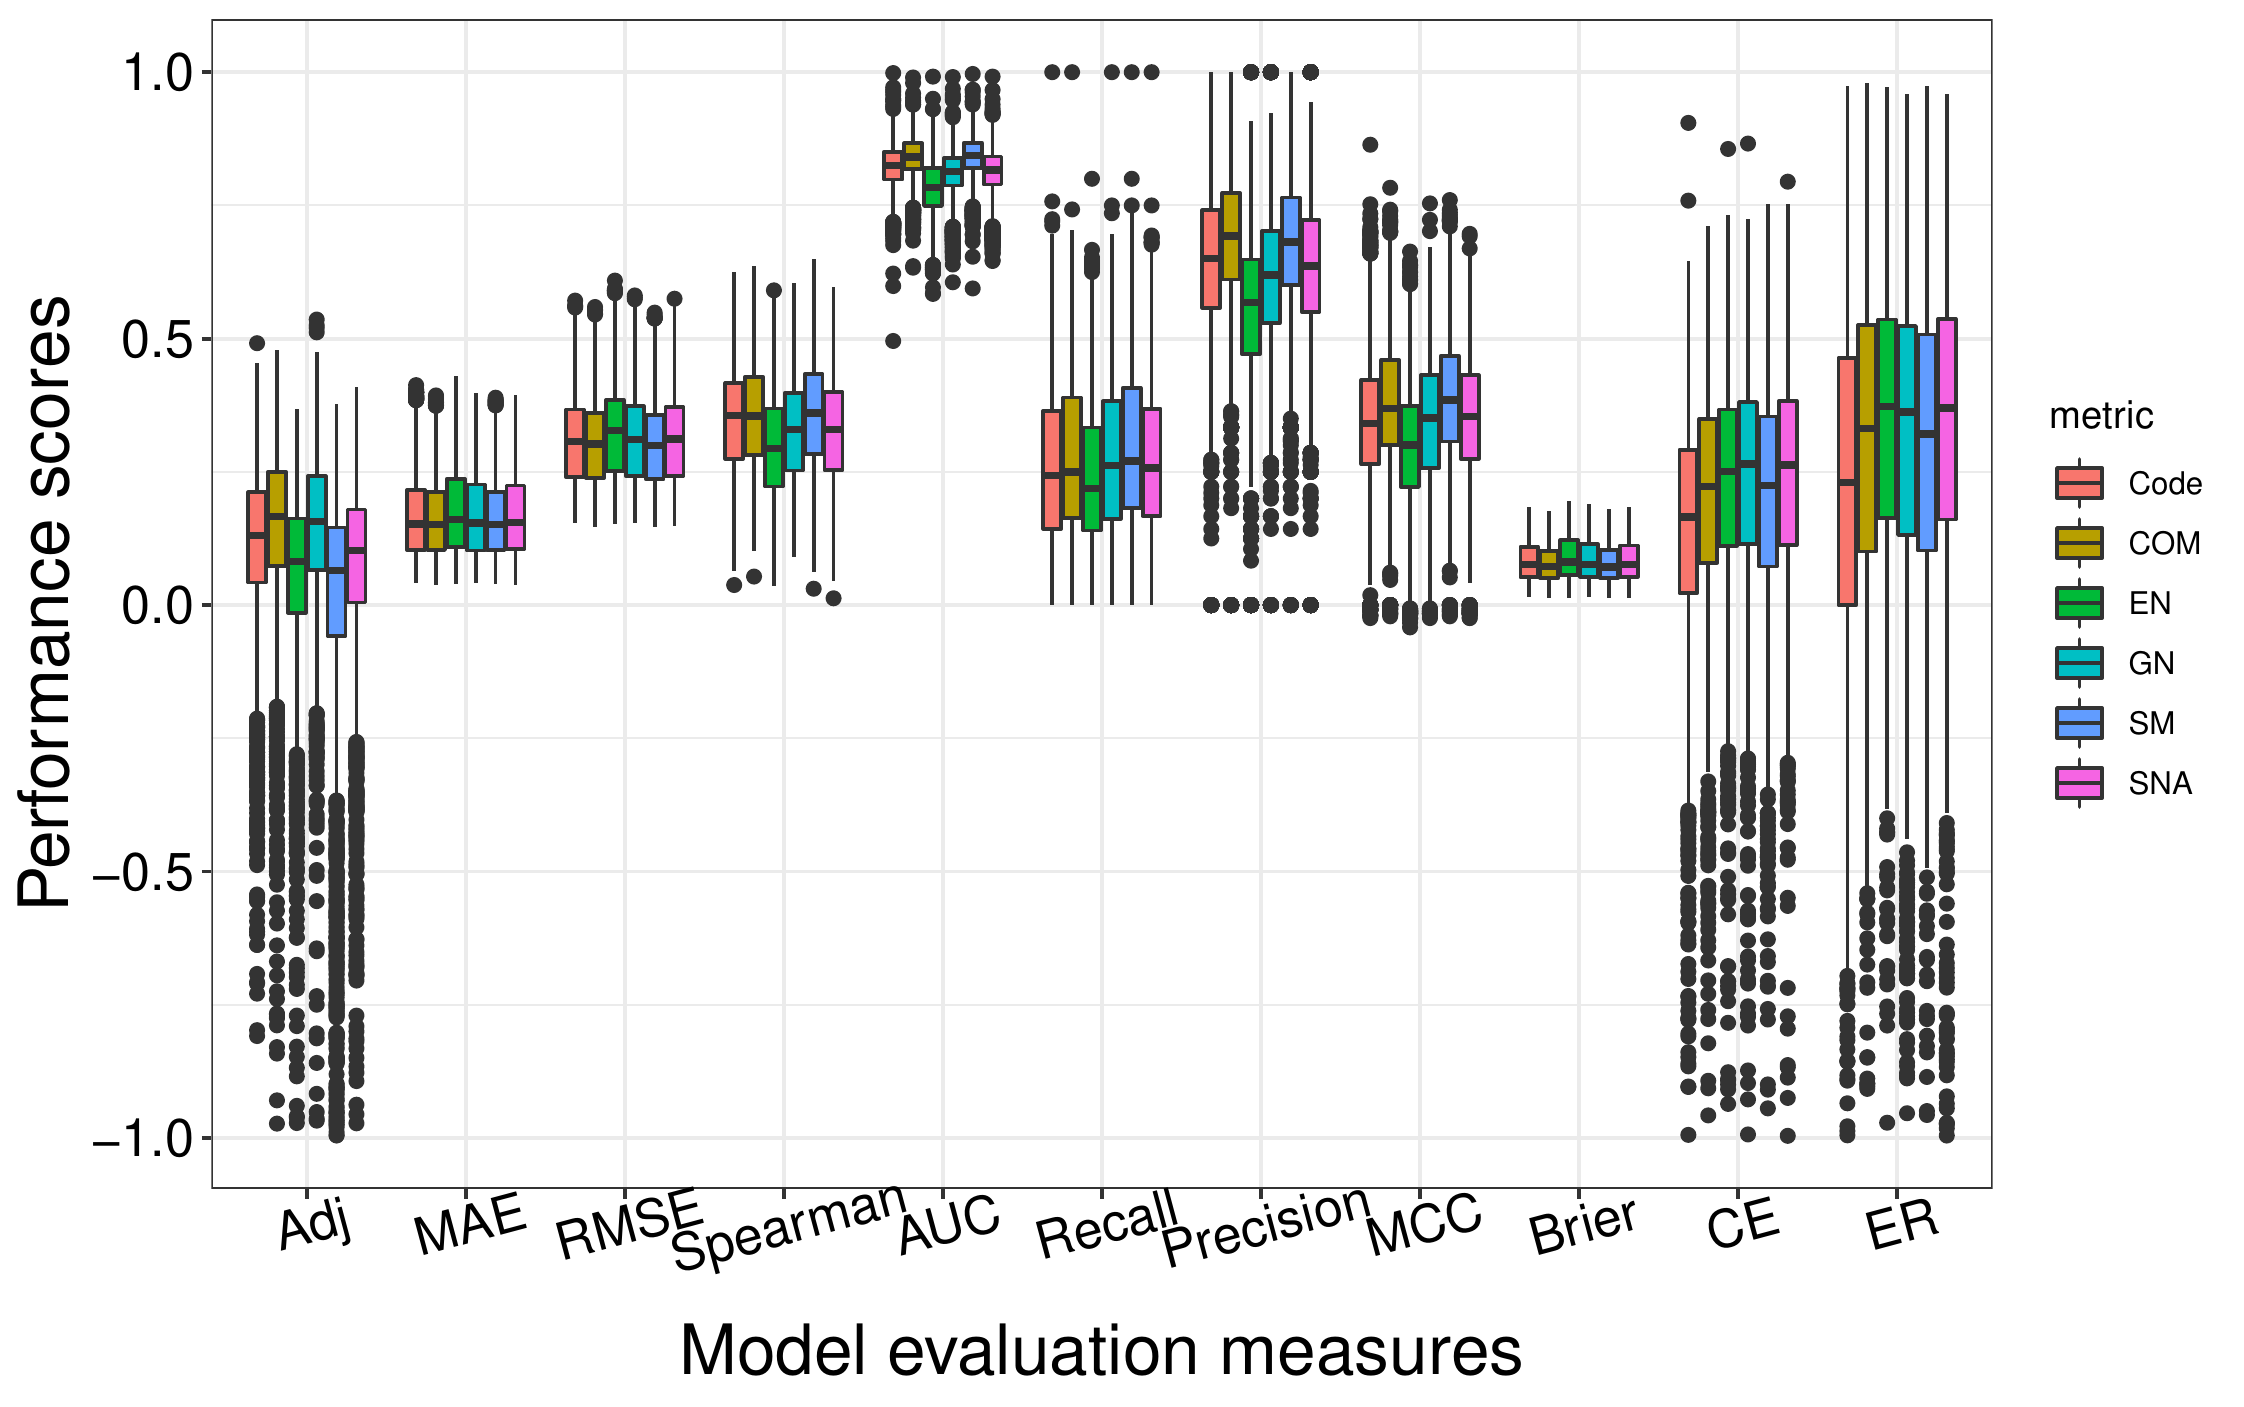}
\caption{Performance of the models trained on the studied metrics in the Within-project context}\label{fig:withip}
\end{figure*}

\section{Performance of the models trained on the studied metrics in the Cross-version context}~\label{sec:app5}
Figure~\ref{fig:crossversion} gives a detailed overview of the performance of models trained on different metric families across the studied datasets for all the SDP scenarios in the Cross-version context.

\begin{figure*}[!htbp]
\centering
\includegraphics[width=7in]{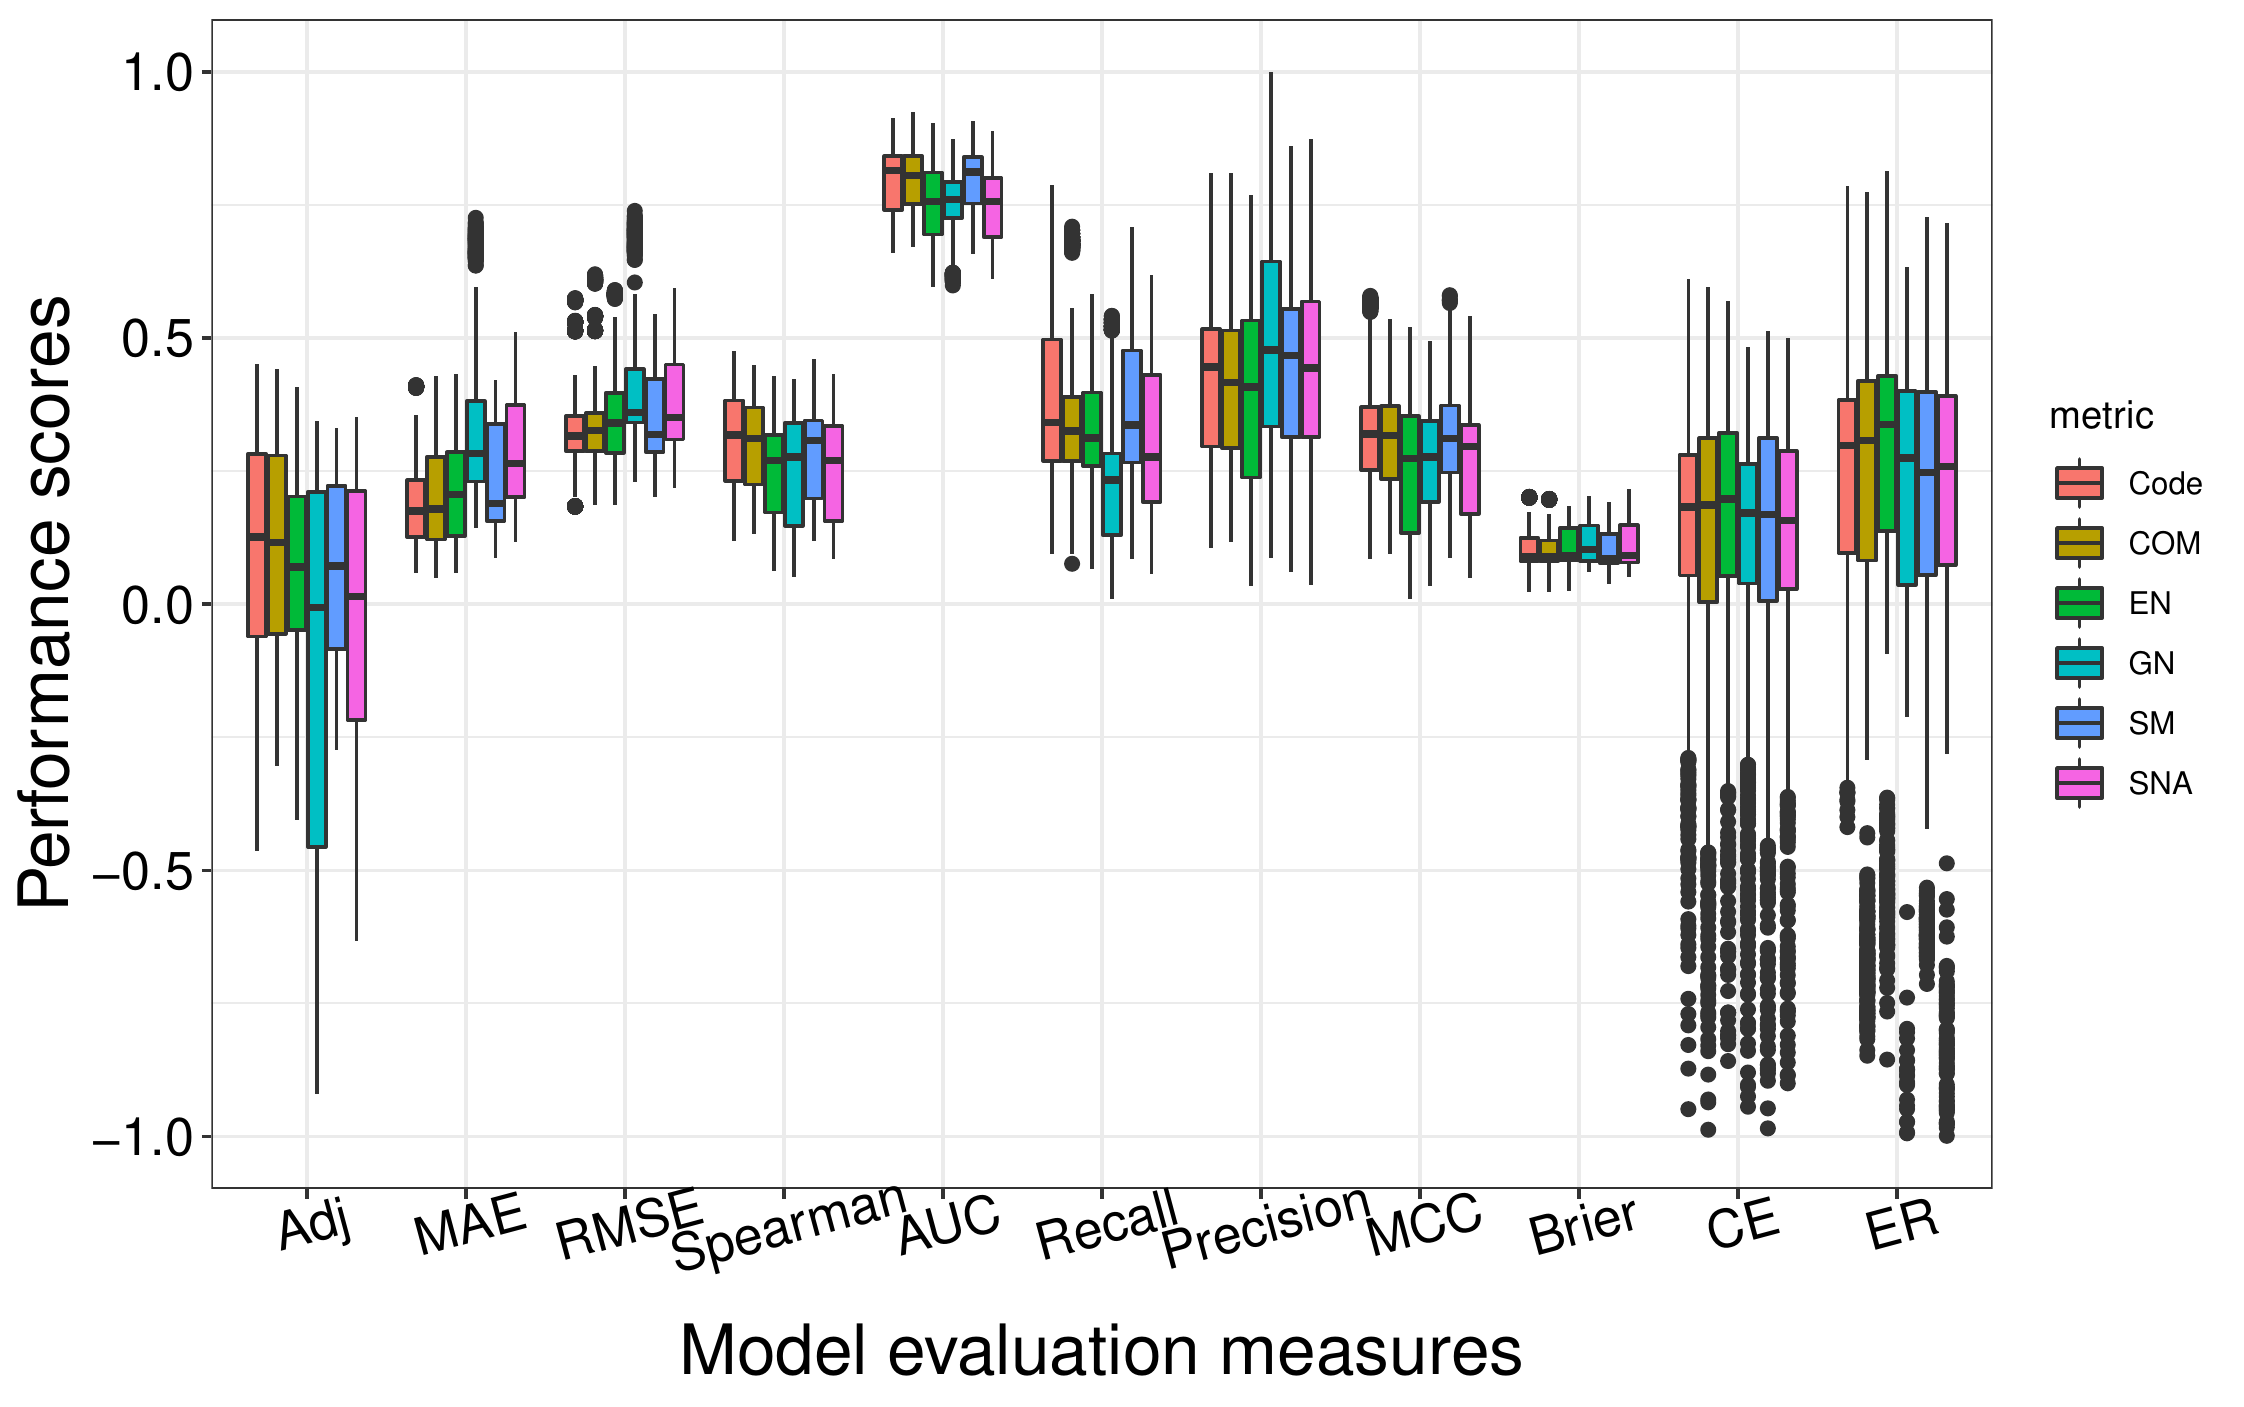}
\caption{Performance of the models trained on the studied metrics in the Cross-version context}\label{fig:crossversion}
\end{figure*}

\section{Performance of the models trained on the studied metrics in the Cross-project context}~\label{sec:app6}
Figure~\ref{fig:crossproject} gives a detailed overview of the performance of models trained on different metric families across the studied datasets for all the SDP scenarios in the Cross-project context.

\begin{figure*}[!htbp]
\centering
\includegraphics[width=7in]{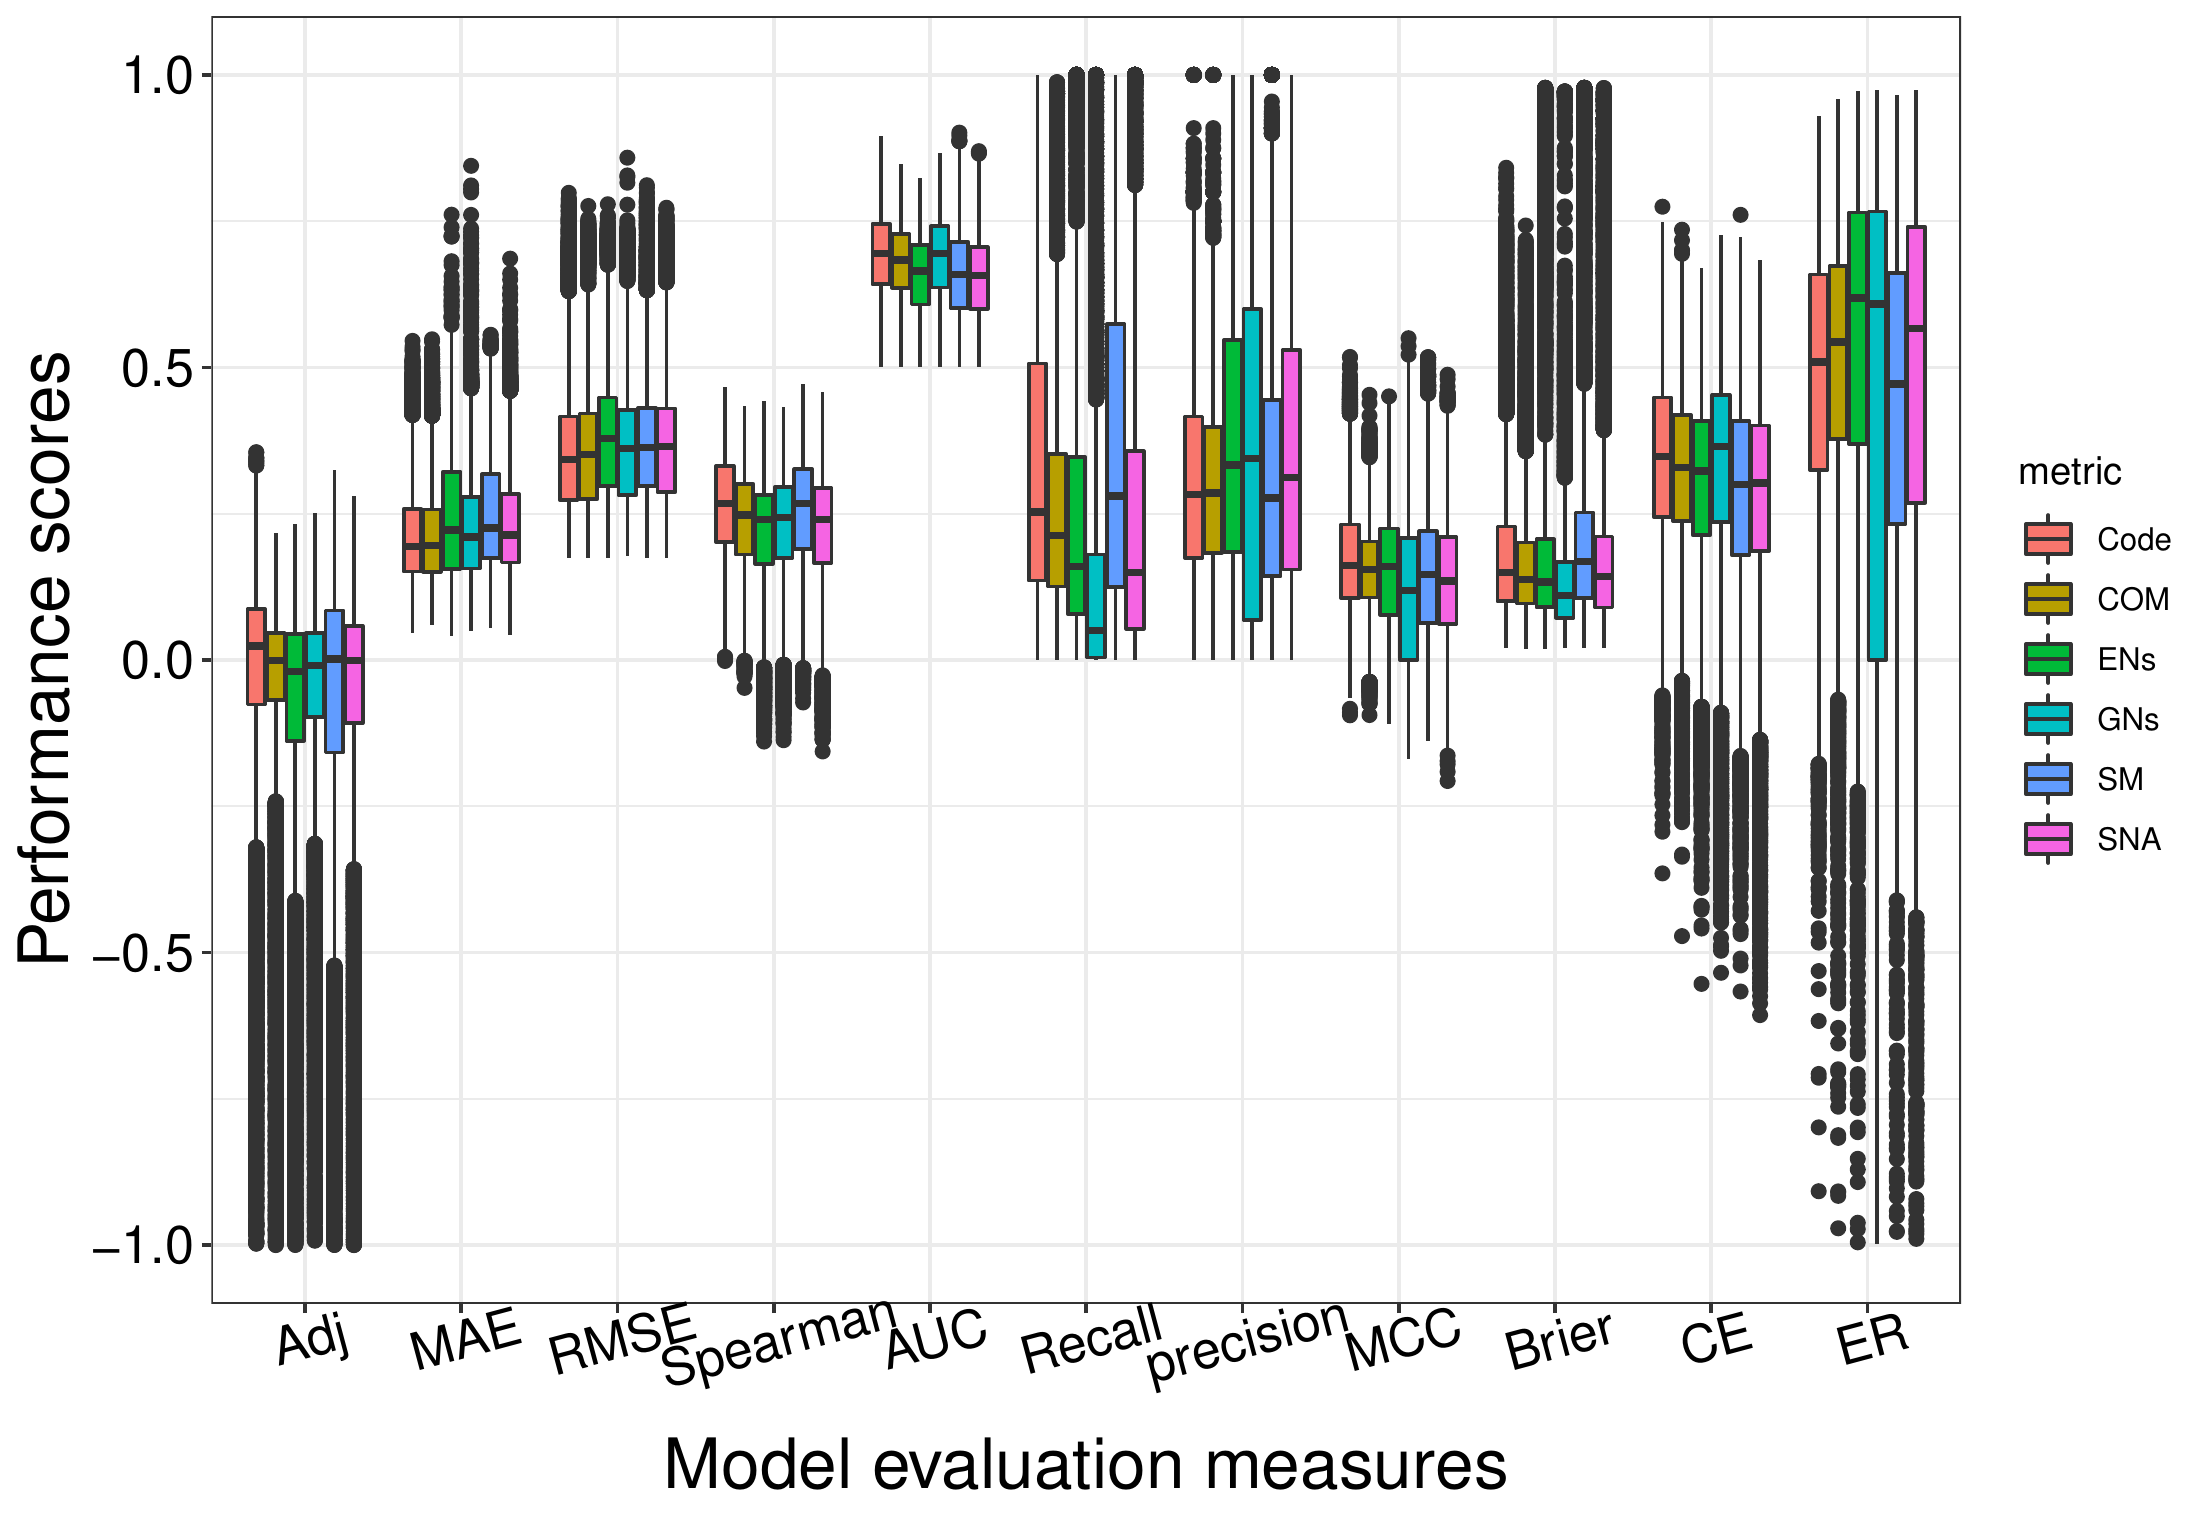}
\caption{Performance of the models trained on the studied metrics in the Cross-project context}\label{fig:crossproject}
\end{figure*}
