# Supplementary material for: Revisiting the Impact of Dependency Network Metrics on Software Defect Prediction
Source: arXiv:2202.06145 source file (2022-02-12)
Supplement: Supplementary file 2 [file 00-appendix-main.tex]

\documentclass[10pt,journal,compsoc]{IEEEtran}
%
% If IEEEtran.cls has not been installed into the LaTeX system files,
% manually specify the path to it like:
% \documentclass[10pt,journal,compsoc]{../sty/IEEEtran}

% Some very useful LaTeX packages include:
% (uncomment the ones you want to load)

% *** MISC UTILITY PACKAGES ***
%
%\usepackage{ifpdf}
% Heiko Oberdiek's ifpdf.sty is very useful if you need conditional
% compilation based on whether the output is pdf or dvi.
% usage:
% \ifpdf
%   % pdf code
% \else
%   % dvi code
% \fi
% The latest version of ifpdf.sty can be obtained from:
% http://www.ctan.org/pkg/ifpdf
% Also, note that IEEEtran.cls V1.7 and later provides a builtin
% \ifCLASSINFOpdf conditional that works the same way.
% When switching from latex to pdflatex and vice-versa, the compiler may
% have to be run twice to clear warning/error messages.

% *** CITATION PACKAGES ***
%
\ifCLASSOPTIONcompsoc
  % IEEE Computer Society needs nocompress option
  % requires cite.sty v4.0 or later (November 2003)
  \usepackage[nocompress]{cite}
\else
  % normal IEEE
  \usepackage{cite}
\fi

\usepackage{xspace}
\usepackage{subfigure}
\usepackage{graphicx}
\usepackage{multirow}
\usepackage{hhline}
\usepackage{comment}
\usepackage{bigstrut}
\usepackage[dvipsnames]{xcolor}
\usepackage[sort&compress,square,comma,numbers]{natbib}
\usepackage[colorlinks=false, linkcolor=blue, citecolor=blue, bookmarks=true,pagebackref=false]{hyperref}
\usepackage{hyphenat}
\usepackage{subcaption}
\usepackage{float}
\usepackage{fancybox}
\usepackage[flushleft]{threeparttable}
\usepackage{array,booktabs}
\usepackage{amsmath}
\usepackage{outlines}
\usepackage[linesnumbered,ruled]{algorithm2e}
\usepackage[misc]{ifsym}
\usepackage{arydshln}
\usepackage{balance}
\usepackage{amsmath}
\usepackage{MnSymbol}
\usepackage{wasysym}
\usepackage{enumitem}
\usepackage{times}
\usepackage{fancyhdr}
\usepackage{courier}
\usepackage{booktabs}
\usepackage{pifont}
\usepackage{color,soul} %Allows text highlighting
\usepackage{tcolorbox}
\usepackage{ragged2e}
\usepackage[justification=centering]{caption}
\usepackage{natbib}
\usepackage{tikz}
\usepackage{capt-of}
% cite.sty was written by Donald Arseneau
% V1.6 and later of IEEEtran pre-defines the format of the cite.sty package
% \cite{} output to follow that of the IEEE. Loading the cite package will
% result in citation numbers being automatically sorted and properly
% "compressed/ranged". e.g., [1], [9], [2], [7], [5], [6] without using
% cite.sty will become [1], [2], [5]--[7], [9] using cite.sty. cite.sty's
% \cite will automatically add leading space, if needed. Use cite.sty's
% noadjust option (cite.sty V3.8 and later) if you want to turn this off
% such as if a citation ever needs to be enclosed in parenthesis.
% cite.sty is already installed on most LaTeX systems. Be sure and use
% version 5.0 (2009-03-20) and later if using hyperref.sty.
% The latest version can be obtained at:
% http://www.ctan.org/pkg/cite
% The documentation is contained in the cite.sty file itself.
%
% Note that some packages require special options to format as the Computer
% Society requires. In particular, Computer Society  papers do not use
% compressed citation ranges as is done in typical IEEE papers
% (e.g., [1]-[4]). Instead, they list every citation separately in order
% (e.g., [1], [2], [3], [4]). To get the latter we need to load the cite
% package with the nocompress option which is supported by cite.sty v4.0
% and later. Note also the use of a CLASSOPTION conditional provided by
% IEEEtran.cls V1.7 and later.

\newtcolorbox{mybox}[2][]{
top=0.15in,left=4pt,right=4pt,bottom=4pt,
fonttitle=\bfseries,
colbacktitle=gray,
colback=gray!5,
colframe=gray!40!black,
enhanced,
attach boxed title to top left={xshift=1.5em,yshift=-\tcboxedtitleheight/2},
boxed title style={size=small},
drop shadow={black!50!white},
title=#2,#1}

 % *** GRAPHICS RELATED PACKAGES ***
%
\ifCLASSINFOpdf
  % \usepackage[pdftex]{graphicx}
  % declare the path(s) where your graphic files are
  % \graphicspath{{../pdf/}{../jpeg/}}
  % and their extensions so you won't have to specify these with
  % every instance of \includegraphics
  % \DeclareGraphicsExtensions{.pdf,.jpeg,.png}
\else
  % or other class option (dvipsone, dvipdf, if not using dvips). graphicx
  % will default to the driver specified in the system graphics.cfg if no
  % driver is specified.
  % \usepackage[dvips]{graphicx}
  % declare the path(s) where your graphic files are
  % \graphicspath{{../eps/}}
  % and their extensions so you won't have to specify these with
  % every instance of \includegraphics
  % \DeclareGraphicsExtensions{.eps}
\fi

% correct bad hyphenation here
\hyphenation{op-tical net-works semi-conduc-tor}

\begin{document}
%
% paper title
% Titles are generally capitalized except for words such as a, an, and, as,
% at, but, by, for, in, nor, of, on, or, the, to and up, which are usually
% not capitalized unless they are the first or last word of the title.
% Linebreaks \\ can be used within to get better formatting as desired.
% Do not put math or special symbols in the title.
\title{Revisiting the Impact of Dependency Network Metrics on Software Defect Prediction - Appendix}
%
%
% author names and IEEE memberships
% note positions of commas and nonbreaking spaces ( ~ ) LaTeX will not break
% a structure at a ~ so this keeps an author's name from being broken across
% two lines.
% use \thanks{} to gain access to the first footnote area
% a separate \thanks must be used for each paragraph as LaTeX2e's \thanks
% was not built to handle multiple paragraphs
%
%
%\IEEEcompsocitemizethanks is a special \thanks that produces the bulleted
% lists the Computer Society journals use for "first footnote" author
% affiliations. Use \IEEEcompsocthanksitem which works much like \item
% for each affiliation group. When not in compsoc mode,
% \IEEEcompsocitemizethanks becomes like \thanks and
% \IEEEcompsocthanksitem becomes a line break with idention. This
% facilitates dual compilation, although admittedly the differences in the
% desired content of \author between the different types of papers makes a
% one-size-fits-all approach a daunting prospect. For instance, compsoc 
% journal papers have the author affiliations above the "Manuscript
% received ..."  text while in non-compsoc journals this is reversed. Sigh.

\author{Lina~Gong,
        Gopi~Krishnan~Rajbahadur,
        ~Ahmed~E.~Hassan, and~Shujuan Jiang% <-this % stops a space
%\IEEEcompsocitemizethanks{\IEEEcompsocthanksitem Lina Gong is with the School of Computer Science and Technology, China University of Mining and Technology, Xuzhou, China and a visitor in the Software Analysis and Intelligence Lab (SAIL), School of Computing, Queen’s University, Canada. E-mail:  linagong@cumt.edu.cn.
% note need leading \protect in front of \\ to get a newline within \thanks as
% \\ is fragile and will error, could use \hfil\break instead.

%\IEEEcompsocthanksitem Gopi~Krishnan~Rajbahadur,
%        and~Ahmed~E.~Hassan are with Software Analysis and Intelligence Lab (SAIL), School of
%Computing, Queen’s University, Canada. E-mail: \{krishnan, ahmed\}@cs.queensu.ca.
%\IEEEcompsocthanksitem Shujuan Jiang is with with the School of Computer Science and Technology, China University of Mining and Technology, Xuzhou, China. E-mail:shjjiang@cumt.edu.cn.
%\IEEEcompsocthanksitem Gopi~Krishnan~Rajbahadur is the corresponding author.
%}% <-this % stops an unwanted space

}

% note the % following the last \IEEEmembership and also \thanks - 
% these prevent an unwanted space from occurring between the last author name
% and the end of the author line. i.e., if you had this:
% 
% \author{....lastname \thanks{...} \thanks{...} }
%                     ^------------^------------^----Do not want these spaces!
%
% a space would be appended to the last name and could cause every name on that
% line to be shifted left slightly. This is one of those "LaTeX things". For
% instance, "\textbf{A} \textbf{B}" will typeset as "A B" not "AB". To get
% "AB" then you have to do: "\textbf{A}\textbf{B}"
% \thanks is no different in this regard, so shield the last } of each \thanks
% that ends a line with a % and do not let a space in before the next \thanks.
% Spaces after \IEEEmembership other than the last one are OK (and needed) as
% you are supposed to have spaces between the names. For what it is worth,
% this is a minor point as most people would not even notice if the said evil
% space somehow managed to creep in.

% The paper headers

\IEEEtitleabstractindextext{%
\begin{abstract}
We provide the supplementary details associated with our study in this appendix to help the readers explore our study better. 
\end{abstract}

% Note that keywords are not normally used for peerreview papers.
%\begin{IEEEkeywords}
%Dependency network metrics, Code metrics, Software defect prediction, Social network analysis (SNA), %Within-project, Cross-version, Cross-project, Effort-aware.
%\end{IEEEkeywords}
}

% make the title area
\maketitle

% To allow for easy dual compilation without having to reenter the
% abstract/keywords data, the \IEEEtitleabstractindextext text will
% not be used in maketitle, but will appear (i.e., to be "transported")
% here as \IEEEdisplaynontitleabstractindextext when the compsoc 
% or transmag modes are not selected <OR> if conference mode is selected 
% - because all conference papers position the abstract like regular
% papers do.
\IEEEdisplaynontitleabstractindextext
% \IEEEdisplaynontitleabstractindextext has no effect when using
% compsoc or transmag under a non-conference mode.

% For peer review papers, you can put extra information on the cover
% page as needed:
% \ifCLASSOPTIONpeerreview
% \begin{center} \bfseries EDICS Category: 3-BBND \end{center}
% \fi
%
% For peerreview papers, this IEEEtran command inserts a page break and
% creates the second title. It will be ignored for other modes.
\IEEEpeerreviewmaketitle

%\IEEEraisesectionheading{\section{Introduction}\label{sec:introduction}}
%\section{Overview of the Double SK-ESD test}~\label{sec:app1}

 % \begin{figure*}[!htbp]
 % \noindent\begin{minipage}{\textwidth}
%\centering

%\includegraphics[angle=90,width=6in]{figures/double_ESD.pdf}
%\caption{Overview of our Double Sk-ESD test}\label{fig:ESD}
%\captionof{figure}{Overview of our Double Sk-ESD test}\label{fig:ESD}
%\end{minipage}
%\end{figure*}

\section{Details about each of the studied SNA metrics}~\label{sec:app1}
Table~\ref{table:SNAmetric} gives a more details about each of the studied SNA metrics used in Section 3.1.2.

\begin{table*}[!htb]
\centering
\caption{Description about each of the studied SNA metrics}\label{table:SNAmetric}
\hspace{0.5cm}
\centering
 \begin{tabular} {l|p{50pt}|p{300pt}} 
\hline
\textbf{Metric family}&\textbf{Measure}&\textbf{Description}\\
\hline
\multirow{12}{*}{\textbf{EN metrics}}&\textbf{Size} & The number of nodes in the ego network of the given module\\
\cline{2-3}
&\textbf{Ties} & The number of edges in the ego network of the given module\\
\cline{2-3}
&\textbf{Pairs} & The number of unique pairs of nodes in ego network of the given module, i.e., $Size \times (Size-1)$\\
\cline{2-3}
&\textbf{Density} & The percentage of possible ties that are actually present, i.e., $Ties/Pairs$\\
\cline{2-3}
&\textbf{WeakComp} & The number of weak components in neighborhood of the given module\\
\cline{2-3}
&\textbf{nWeakComp} & The number of weak components normalized by size of the module, i.e., $WeakComp/Size$\\
\cline{2-3}
&\textbf{2StepReach} & The percentage of nodes that are reachable within two steps from the given node in a ego network\\
\cline{2-3}
&\textbf{ReachEfficency} & Normalize 2StepReach by Size, i.e., $2StepReach/Size$ \\
\cline{2-3}
&\textbf{Brokerage} & The number of pairs that are not directly connected to the given module.\\
\cline{2-3}
&\textbf{nBrokerage} & Normalize Brokerage by the number of pairs, i.e.,$Brokerage/Pairs$\\
\cline{2-3}
&\textbf{EgoBetween} & The percentage of shortest paths between any two nodes in the ego network \\
\cline{2-3}
&\textbf{nEgoBetween} & Normalize Betweenness  by the size of the ego network of the given node.\\
\hline
\multirow{11}{*}{\textbf{GN metrics}}&\textbf{Degree} & The number of nodes that are directly connected to a given node.\\
\cline{2-3}
&\textbf{Eigenvector} & Assign relative scores to all nodes in the dependency graphs similar to Google's PageRank. The node that is connected to many highly connected neighbours would have higher value and vice versa.\\
\cline{2-3}
&\textbf{power} & A modification of the degree of centrality measure, which measures the connections of the nodes in its neighborhood.\\
\cline{2-3}
&\textbf{Closeness} & Sum of the lengths of the shortest paths from a node to all other nodes in the Global network. \\
\cline{2-3}
&\textbf{Betweenness} & Measures how often a node occurs in shortest paths between any two nodes in the Global network.\\
\cline{2-3}
&\textbf{Information} & The harmonic mean of the length of all paths leading to the node.\\
\cline{2-3}
&\textbf{dwReach} & The number of nodes that can be reached from a node. \\
\cline{2-3}
&\textbf{EffSize} & The number of nodes that are connected to a node minus the average number of ties between these nodes.\\
\cline{2-3}
&\textbf{Efficiency} & Normalize EffSize to the total size of the global network.\\
\cline{2-3}
&\textbf{Constraint} & Measures the extent to which the node is limited in options to reach other nodes.\\
\cline{2-3}
&\textbf{Hierarchy} & Measures the concentration of constraint in the global network.\\
\hline
\end{tabular}
\end{table*}

\section{Performance measures used in the Defect-classification scenario}~\label{sec:app2}
Table~\ref{table:measures} presents a detailed description about each of the studied performance measure used in Section 3.3.2.

\begin{table*}[!htb]
\centering
\caption{Performance measures used in our study on the Defect-classification scenario}\label{table:measures}
\hspace{0.5cm}
\centering
 \begin{tabular} {l|p{180pt}|p{200pt}} 
\hline
\textbf{Measure}&\textbf{Definition}&\textbf{Description}\\
\hline
AUC&The  area  under  the  receiver  operator  characteristic  Curve.& The  receiver  operator  characteristic  Curve plots the true positive rate against the false positive rate across all the thresholds\\
Recall&$Recall=\frac{TP}{TP+FN}$& The percentage of defective modules that are correctly classified as defective.\\
Precision&$Precision=\frac{TP}{TP+FP}$&The percentage of predicted defective modules that are actually defective.\\
MCC&$MCC=\frac{TP\times TN-FP\times FN}{(TP+FP)(TP+FN)(TN+FP)(TN+FN)}$& A more balanced indicator which considers TP, TN, FP and FN.\\
Brier score&$Brier=\frac{1}{N}\sum_{i=1}^{N}(p_{i}-y_{i})^{2}$&A measure of the  mean  squared  difference  between  the  predicted  probability assigned  to a module and the actual probability.\\
\hline
\end{tabular}
\end{table*}

\section{Performance of the models trained on the studied metrics in the Within-project context}~\label{sec:app3}
Figure~\ref{fig:withip} gives a detailed overview of the performance of models trained on different metric families across the studied datasets for all the SDP scenarios in the Within-project context.

\begin{figure*}[!htbp]
\centering
\includegraphics[width=7in]{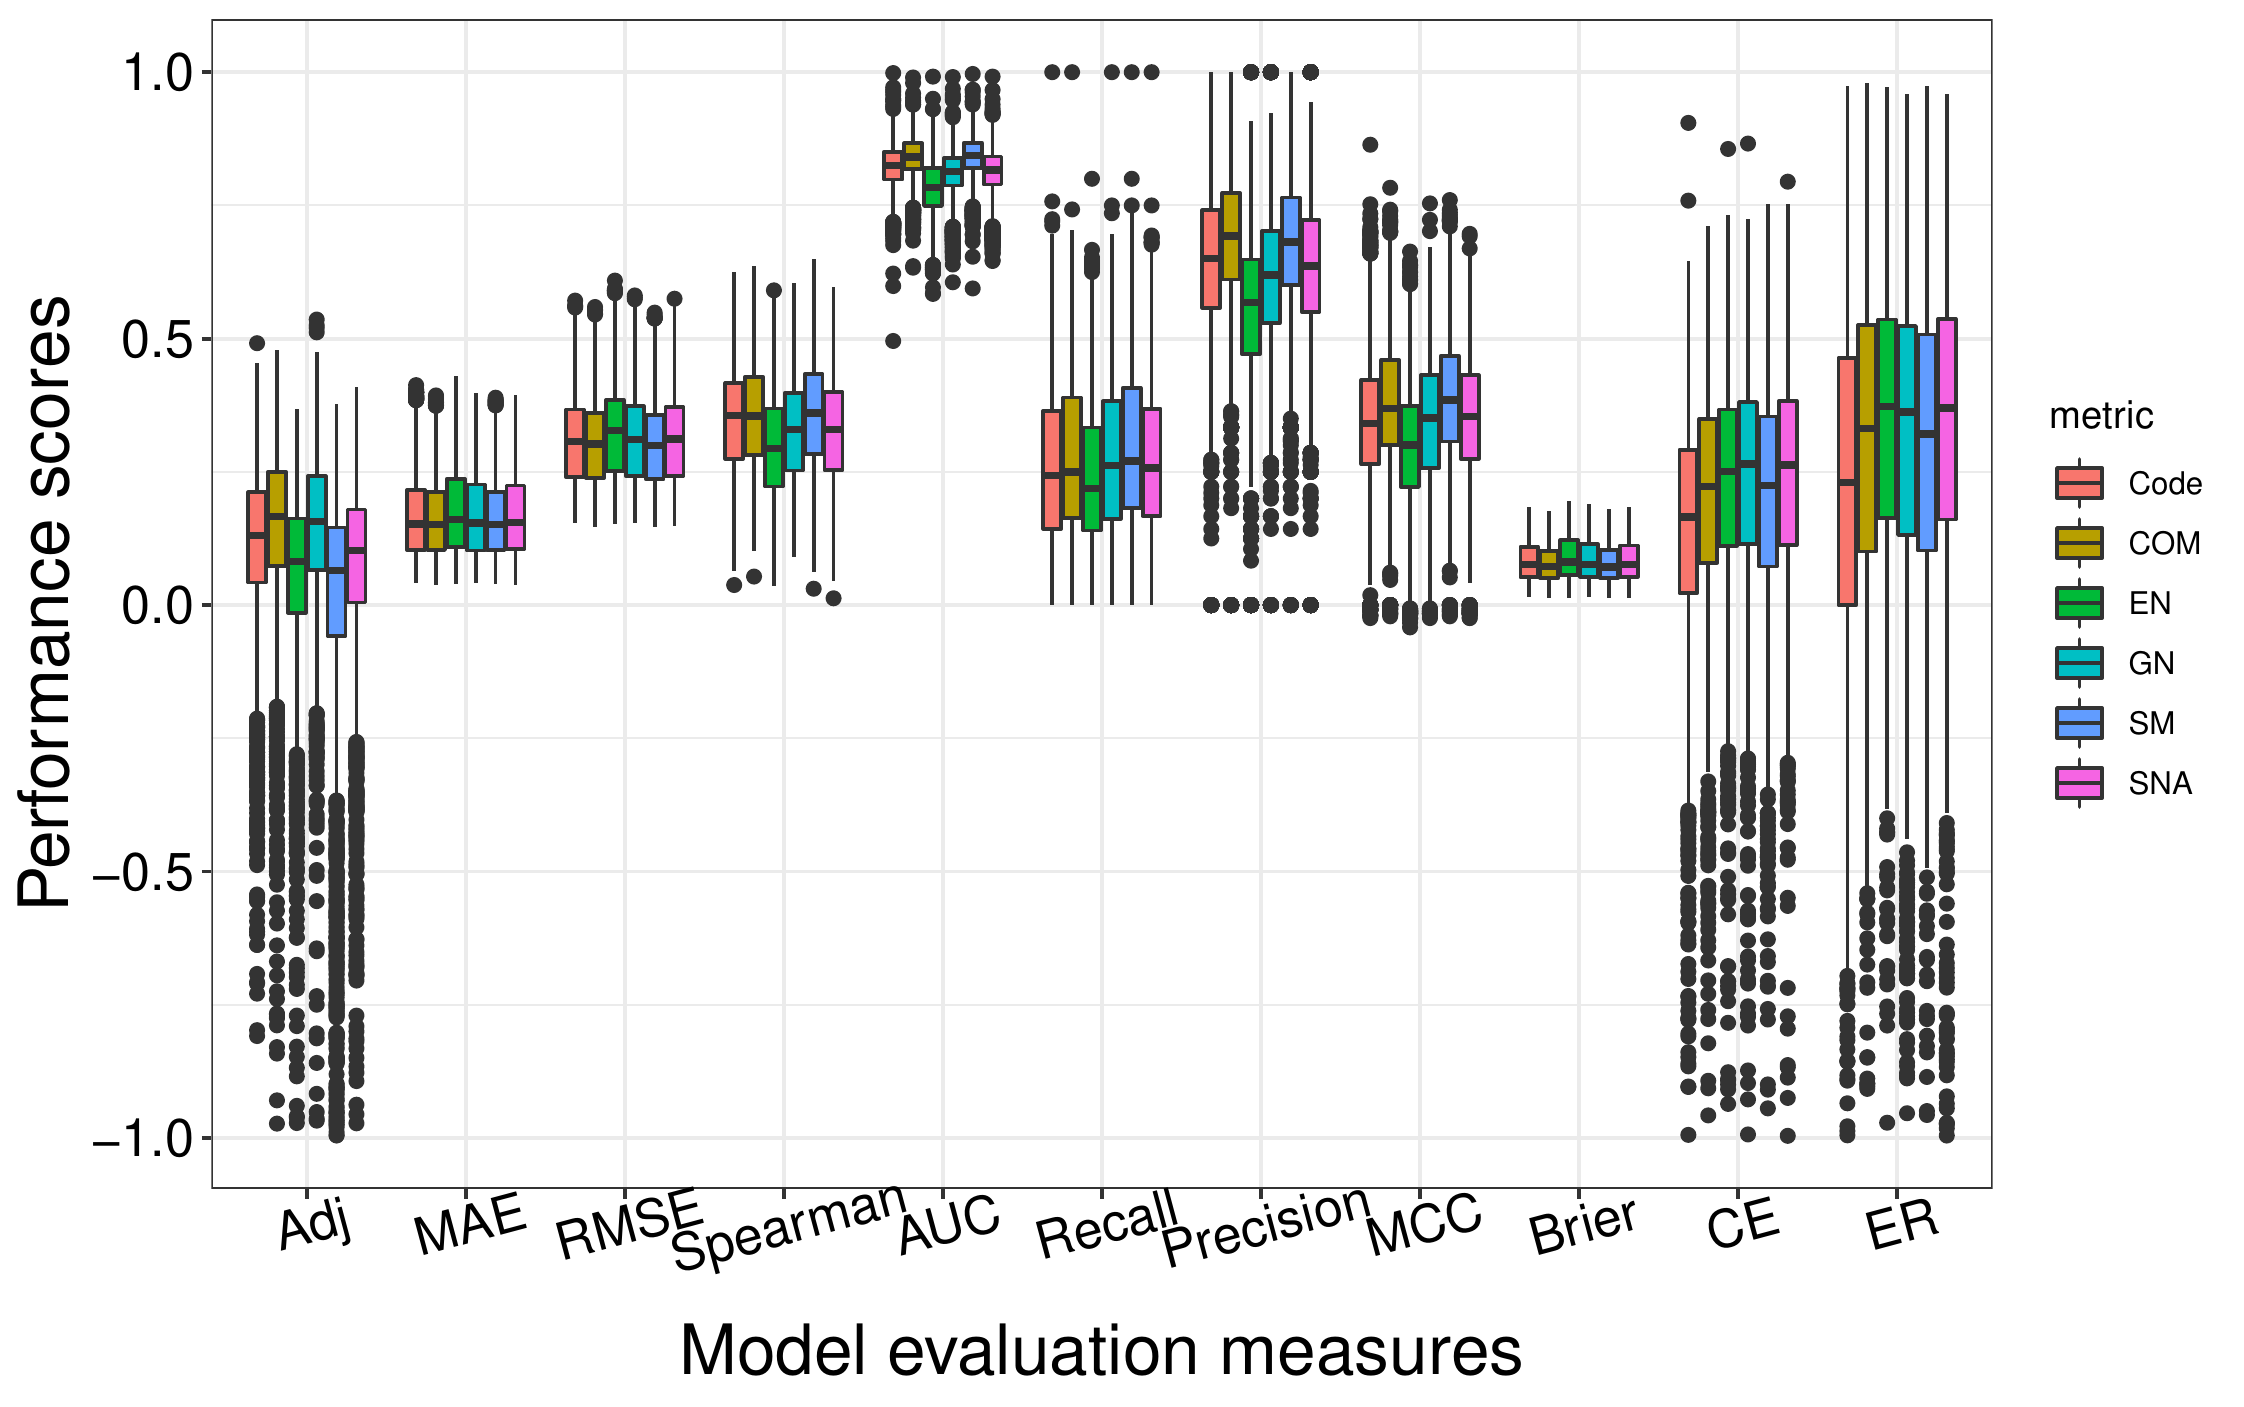}
\caption{Performance of the models trained on the studied metrics in the Within-project context}\label{fig:withip}
\end{figure*}

\section{Performance of the models trained on the studied metrics in the Cross-version context}~\label{sec:app5}
Figure~\ref{fig:crossversion} gives a detailed overview of the performance of models trained on different metric families across the studied datasets for all the SDP scenarios in the Cross-version context.

\begin{figure*}[!htbp]
\centering
\includegraphics[width=7in]{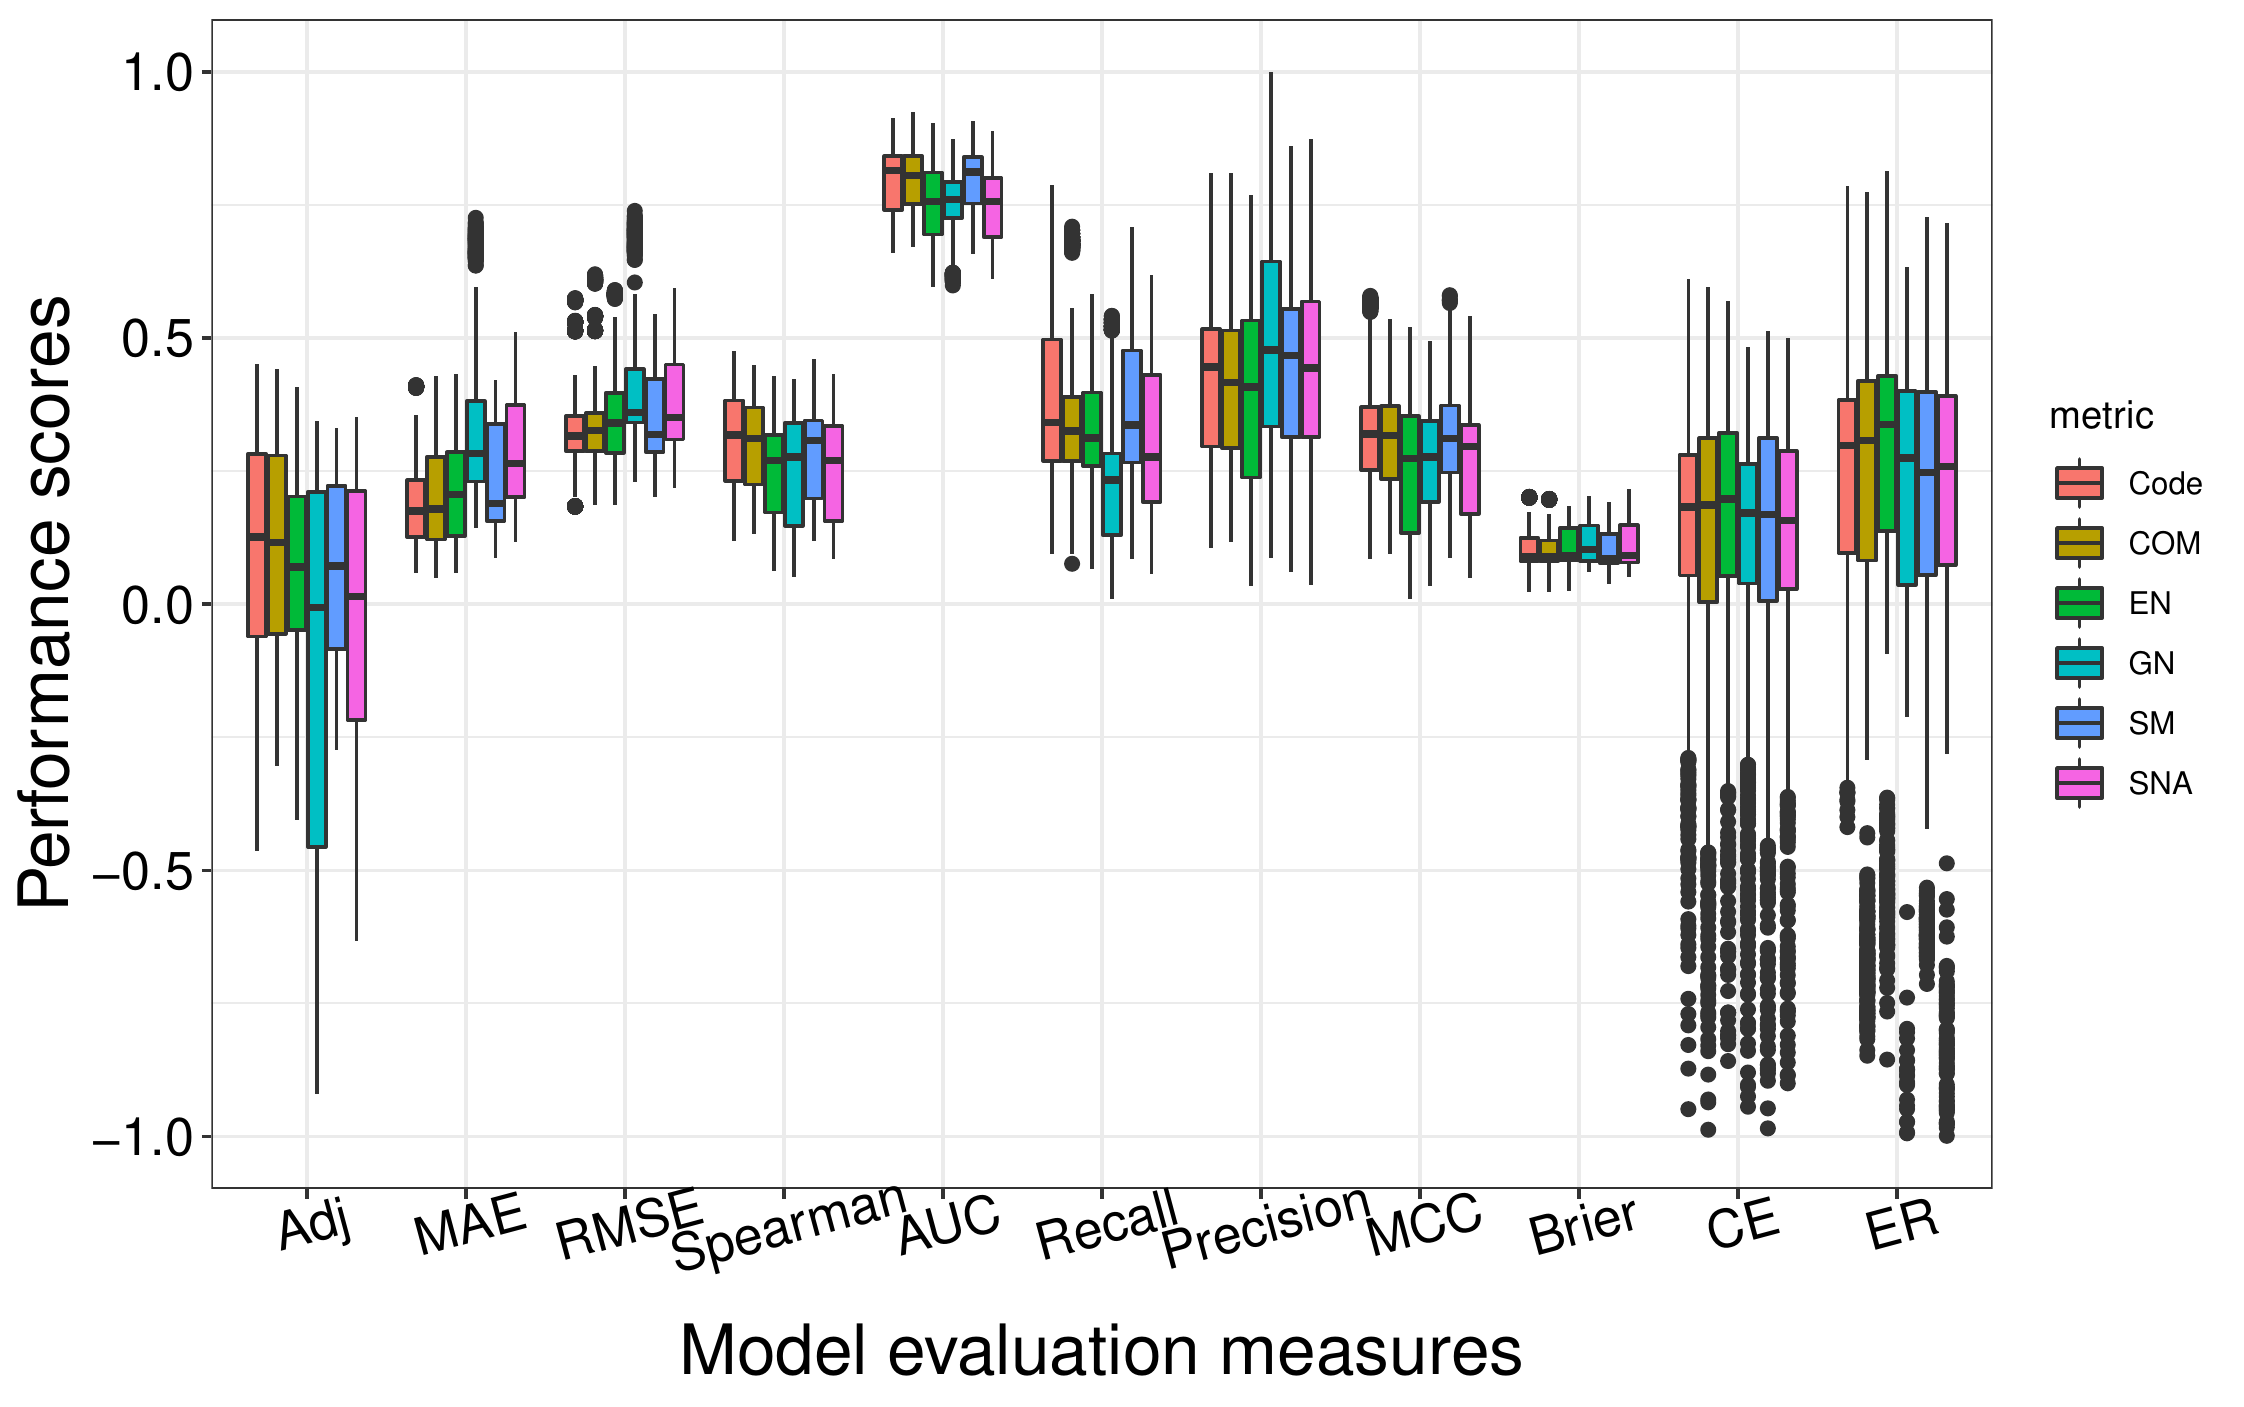}
\caption{Performance of the models trained on the studied metrics in the Cross-version context}\label{fig:crossversion}
\end{figure*}

\section{Performance of the models trained on the studied metrics in the Cross-project context}~\label{sec:app6}
Figure~\ref{fig:crossproject} gives a detailed overview of the performance of models trained on different metric families across the studied datasets for all the SDP scenarios in the Cross-project context.

\begin{figure*}[!htbp]
\centering
\includegraphics[width=7in]{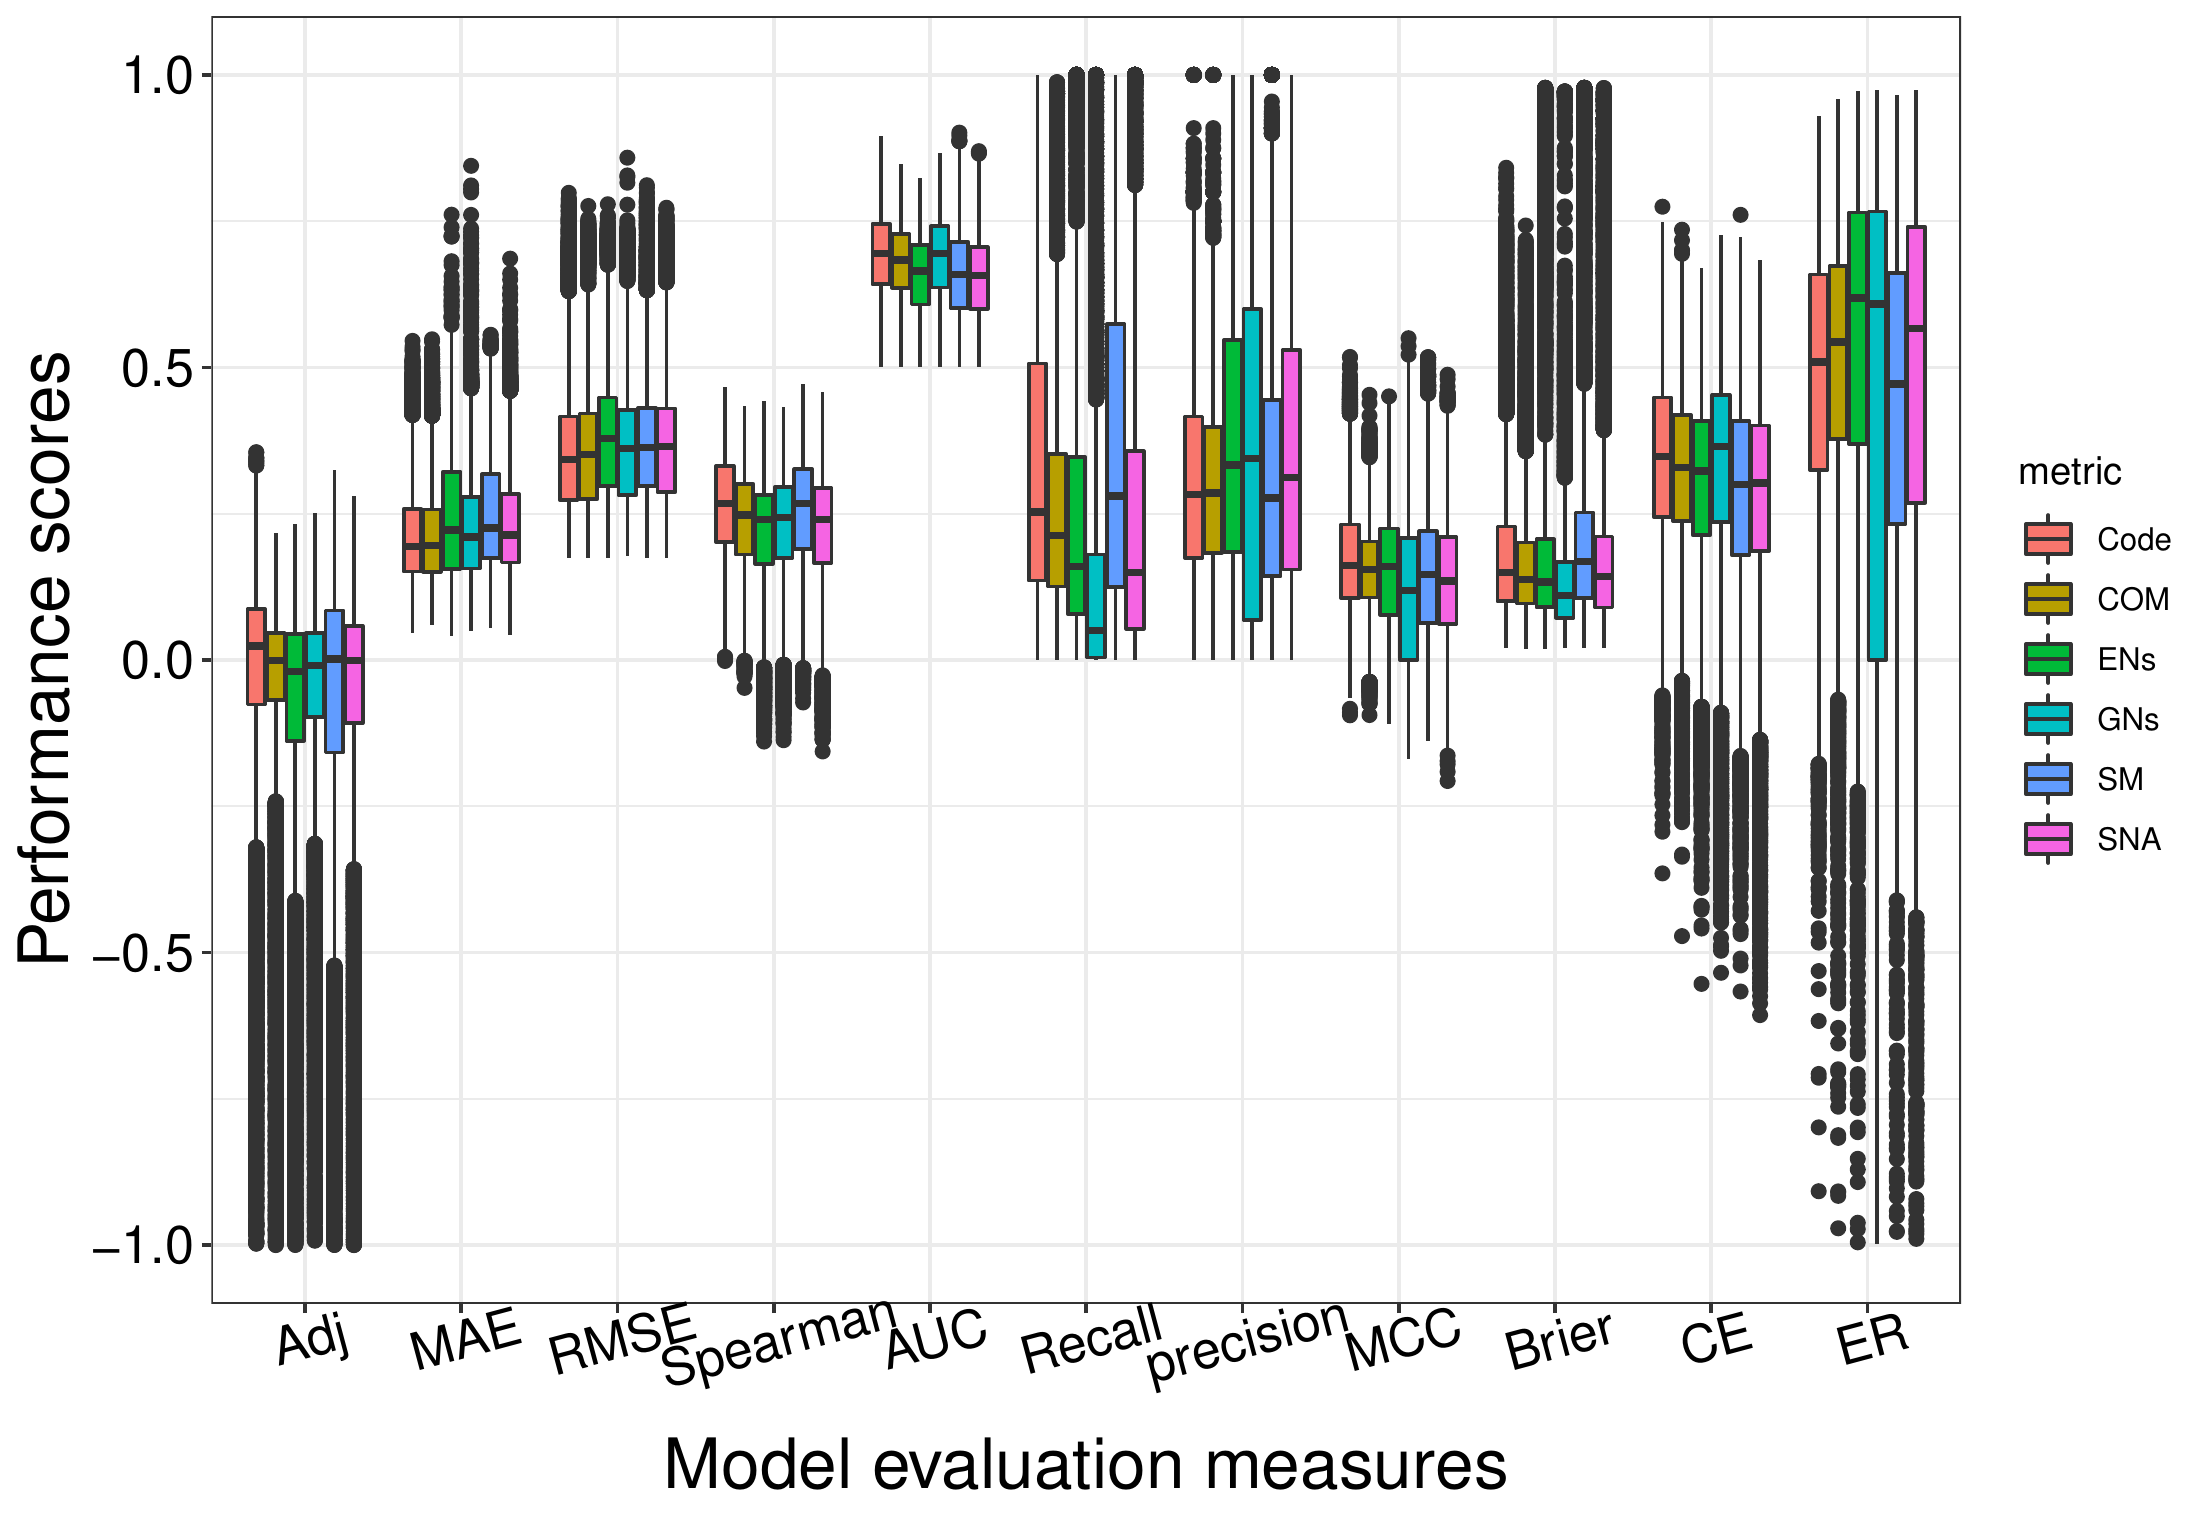}
\caption{Performance of the models trained on the studied metrics in the Cross-project context}\label{fig:crossproject}
\end{figure*}
\iffalse
\input{02-Introduction.tex}
\input{03-Related_works.tex}
\input{04-Background.tex}
\input{05-Study_design.tex}
\input{06-Case_study_results.tex}
\input{07-implications.tex}
\input{08-Threats_to_validity.tex}
\input{09-Conclusion.tex}

% use section* for acknowledgment
\ifCLASSOPTIONcompsoc
  % The Computer Society usually uses the plural form
  \section*{Acknowledgments}
\else
  % regular IEEE prefers the singular form
  \section*{Acknowledgment}
\fi

This paper would not have been possible without the generous support by joint Ph.D. program of “double first rate” construction disciplines of CUMT.

% Can use something like this to put references on a page
% by themselves when using endfloat and the captionsoff option.
\ifCLASSOPTIONcaptionsoff
  \newpage
\fi

\bibliographystyle{IEEEtranSN}
% argument is your BibTeX string definitions and bibliography database(s)
\begin{footnotesize}
\balance
\bibliography{bibliography}
\end{footnotesize}
%
\input{bios}
\newpage
\fi
%\begin{appendices}
% \input{appendix}

%\end{appendices}

\end{document}
